# Supplementary material for: A deep-learning-based surrogate model for data assimilation in dynamic subsurface flow problems
Source: arXiv:1908.05823 source file (2019-08-16)
Supplement: Supplementary file 1 [file appendix.tex]

\section*{Appendix}

\begin{figure}[htbp]
  \centering
  \includegraphics[width=\linewidth]{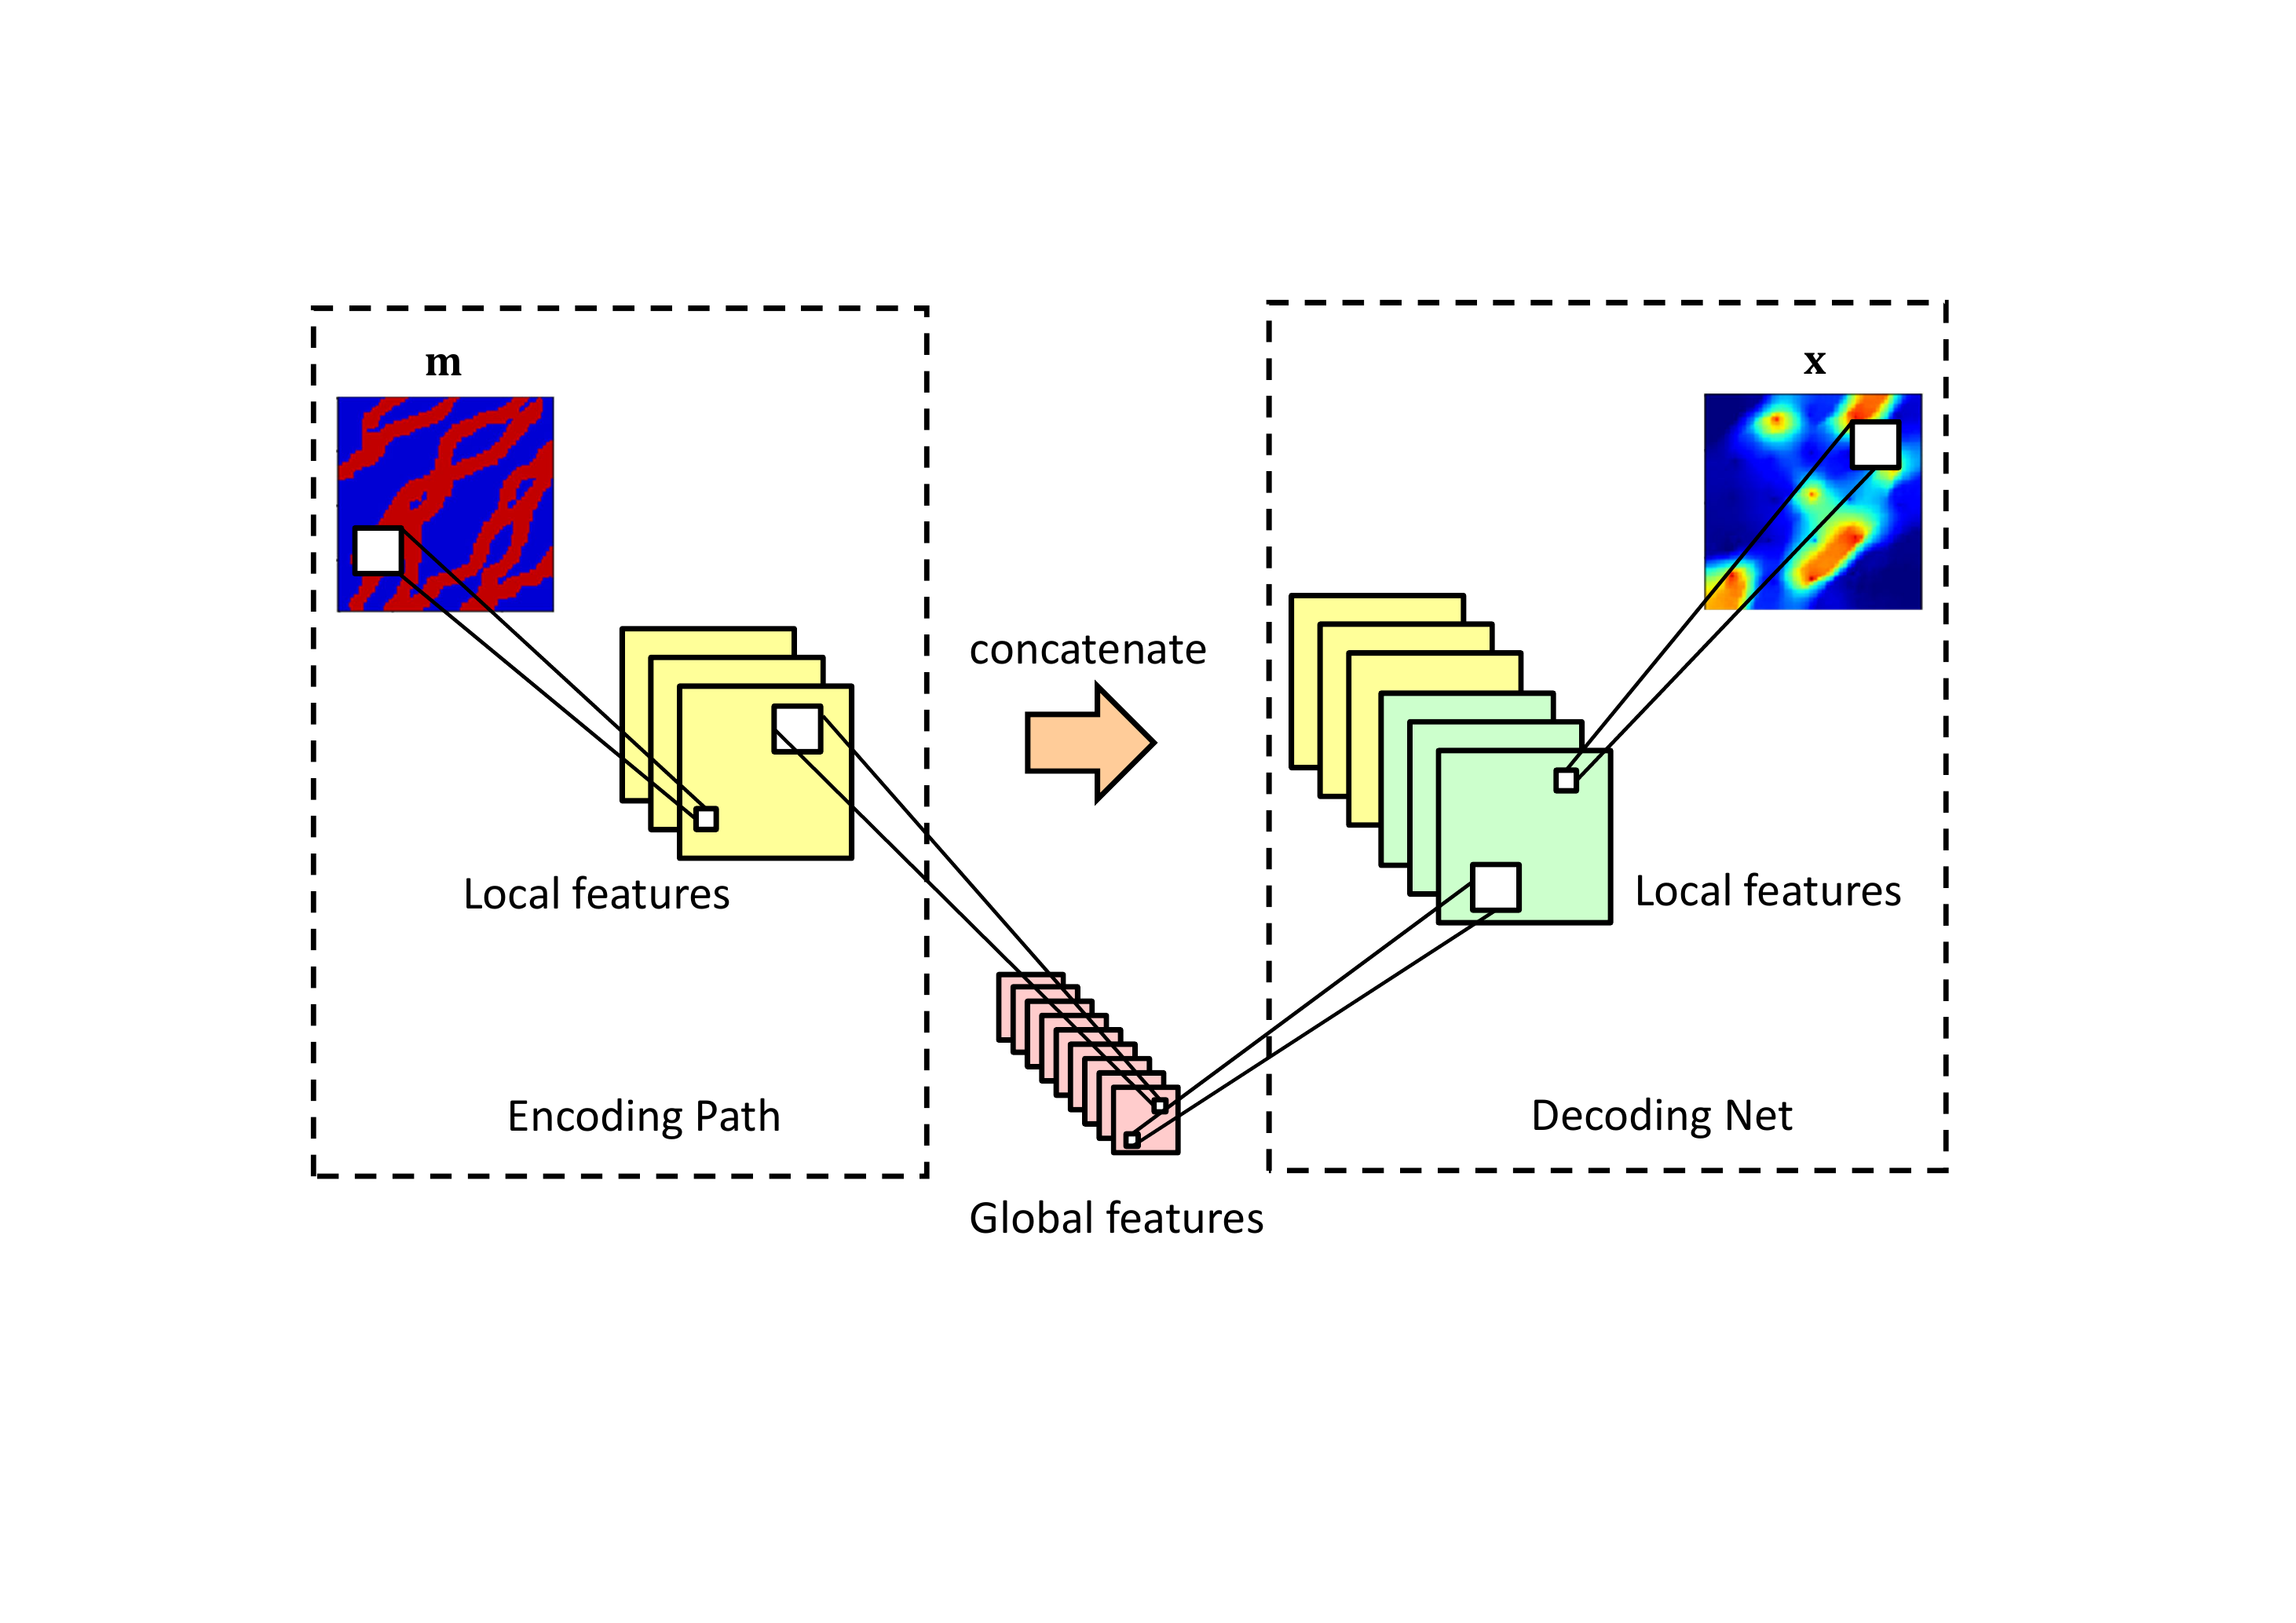}
  \caption{Residual U-Net. }
  \label{fig:r-u-net}
\end{figure}

In Fig.~\ref{fig:r-u-net}, blocks represents the feature (or input and output) maps. The number on top of each feature map (e.g., 128) depicts the number of channels~(depth), and the number in the front of each feature map (e.g., $20 \times 20$) depicts the feature map size. The arrows with different colors represent different operations performed in R-U-Net, where, specifically, blue arrows denote the convolution operation with kernel size $3\times3$ and stride $3\times3$, followed by batch normalization~(BN)~\citep{ioffe2015batch} and rectified linear unit~(ReLU)~\citep{nair2010rectified}, red arrows denote the convolution operation with kernel size $3\times3$ and stride $1\times1$ followed by BN and ReLU, yellow arrows represent the transposed convolution operation~\citep{dumoulin2016guide} with kernel size $3\times3$ and stride $3\times3$, blue arrows represent the transposed convolution operation with kernel size $3\times3$ and stride $1\times1$, grey arrows depict the copy and concatenation of feature maps in the encoding path to the decoding path, and yellow arrows depict residual blocks whose details are shown in Fig.~\ref{fig:residual-block}.

\begin{figure}[htbp]
  \centering
  \includegraphics[width=\linewidth]{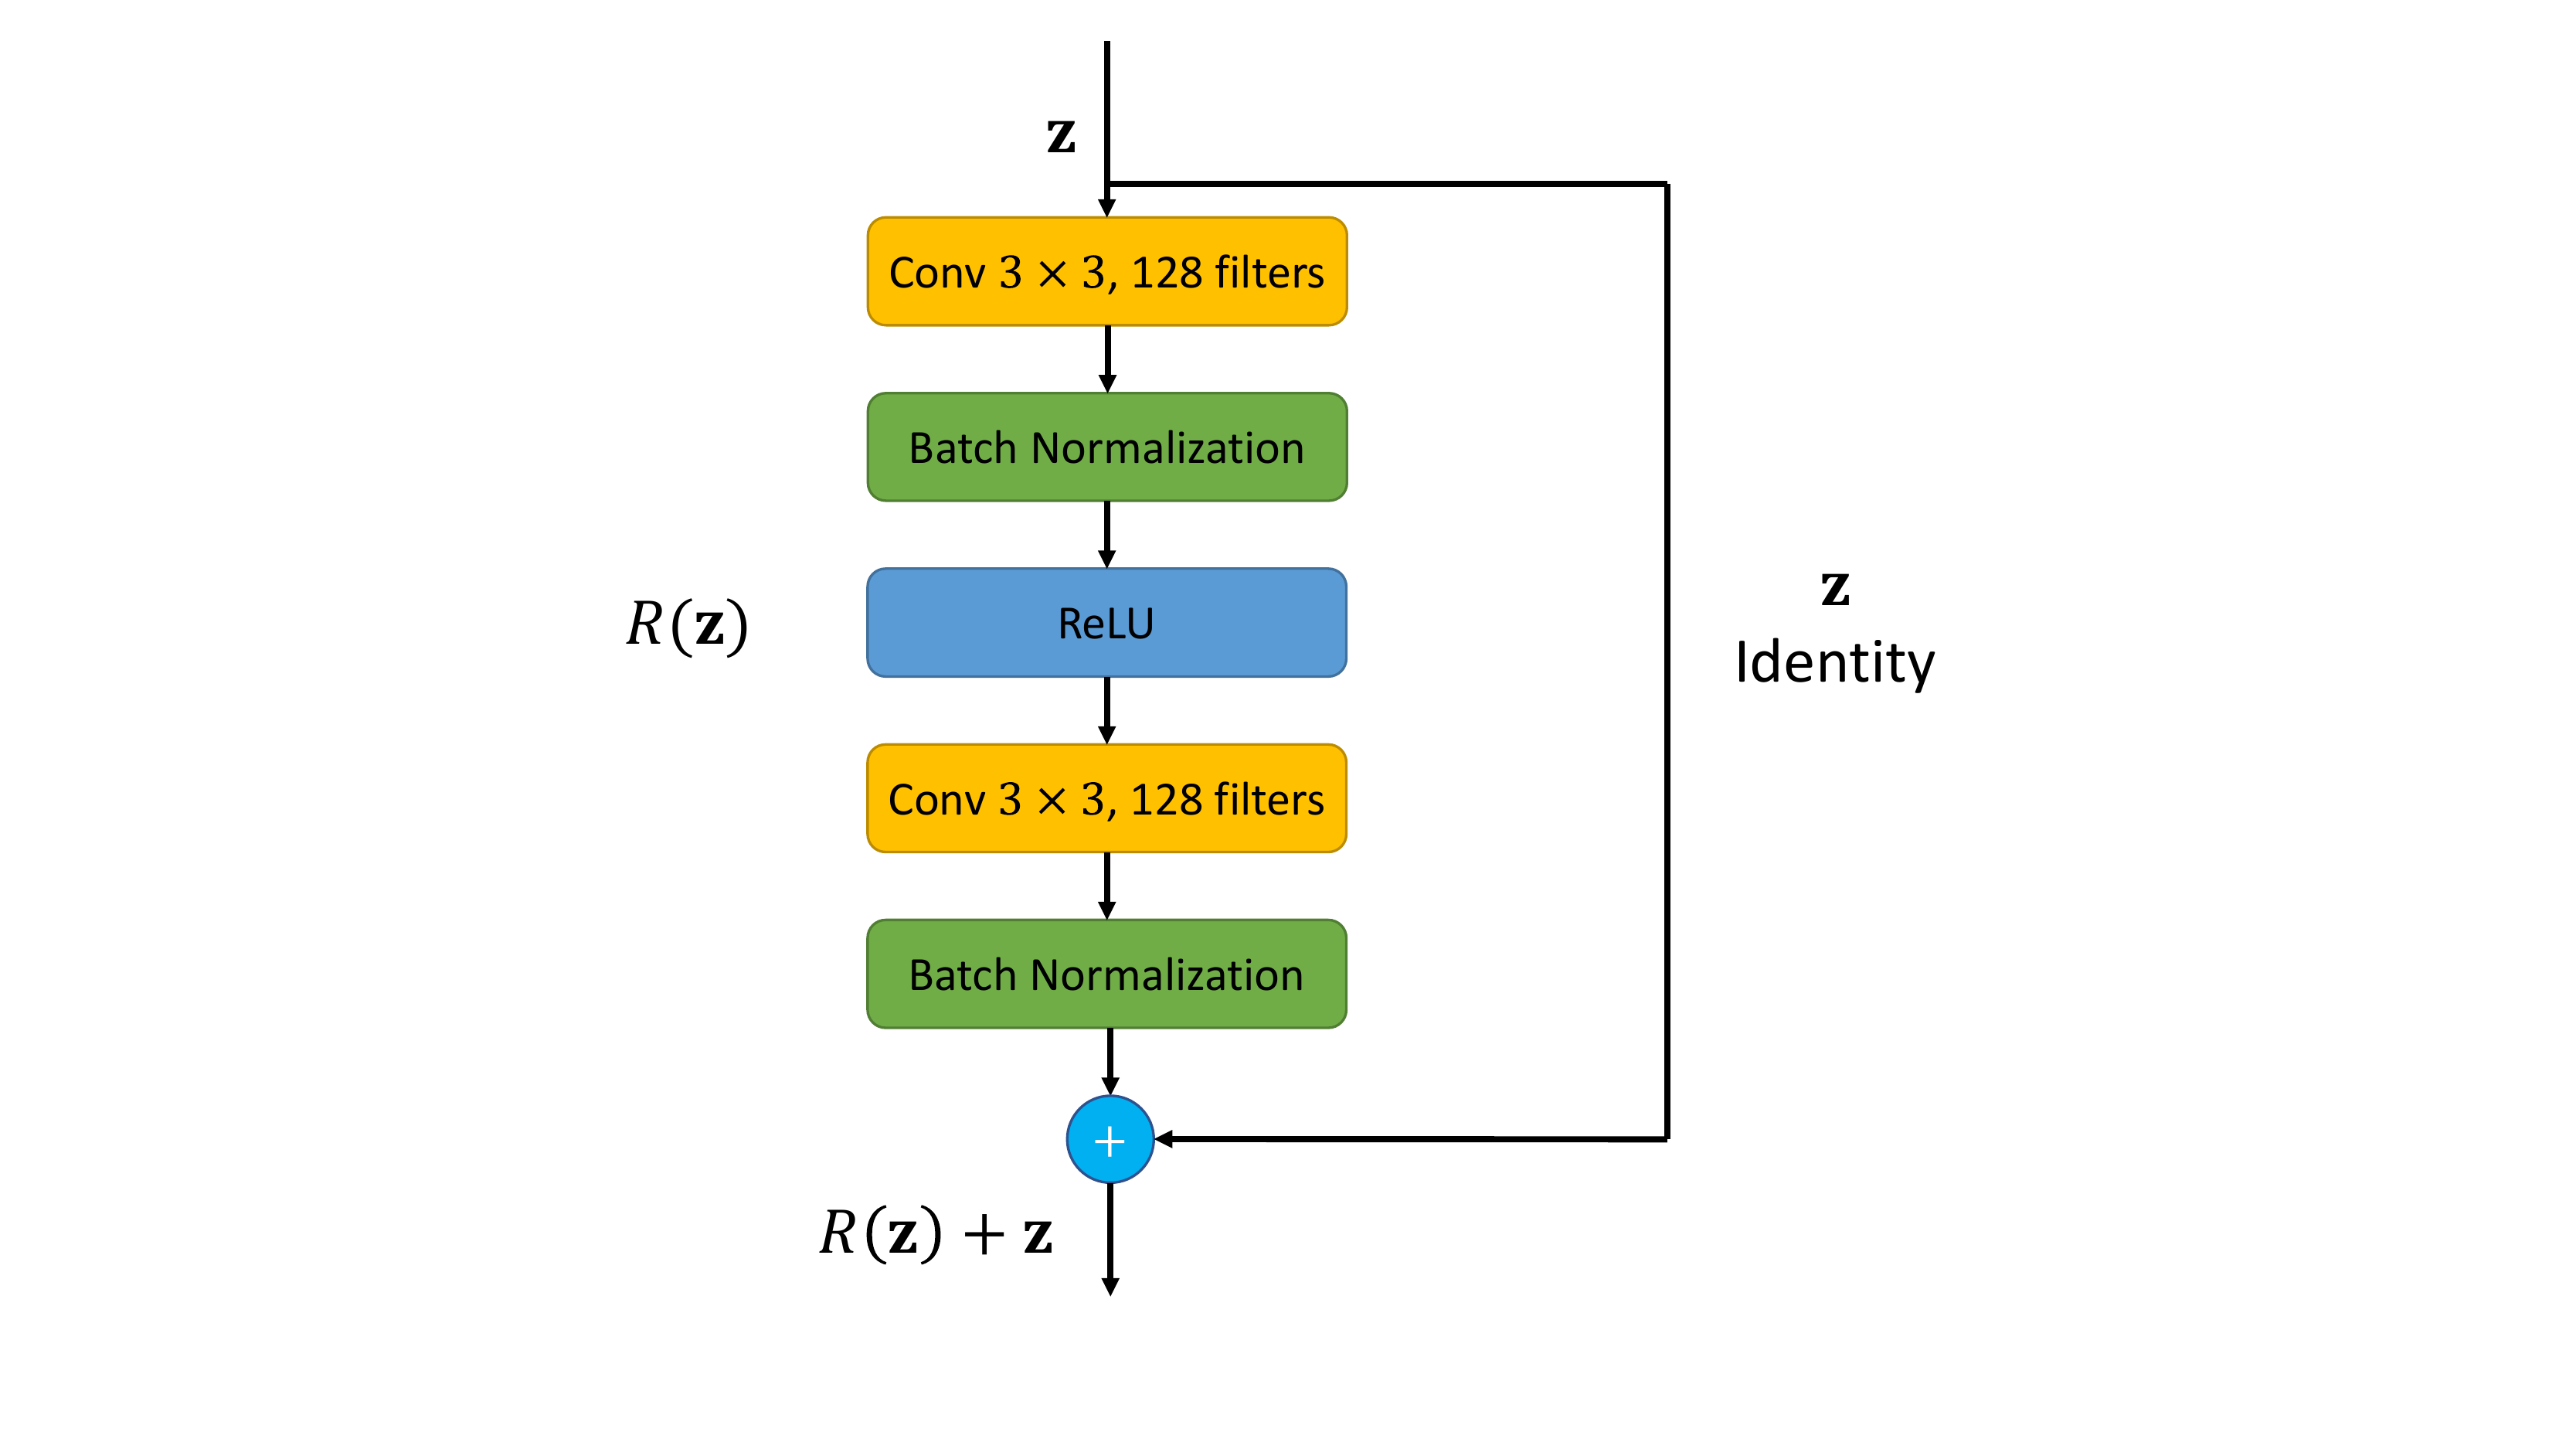}
  \caption{Residual U-Net. }
  \label{fig:residual-block}
\end{figure}

Residual blocks improve the information flow locally during training by adding the identity mapping of input features $\mathbf{z}$ to the output of stacked layers $R(\mathbf{z})$, and the arrows in Fig.~\ref{fig:residual-block} depict the information flow directions.
